# Supplementary material for: Function based sim-to-real learning for shape control of deformable free-form surfaces
Source: arXiv:2405.08935 source file (2024-05-14)
Supplement: Supplementary file 1 [file secAppendix.tex]

\appendix
\subsection{Differentiation of Shape Approximation Loss}
\label{Appendix:GradCompShapeLoss}

For Equ.\ref{eqLoss}, we want to calculate the gradient of the shape approximation loss $D(\mathcal{T}(\mathbf{R},\mathbf{t}),\mathcal{S}(\mathbf{a}))$
with respect to actuation parameter $\mathbf{a}$:

\begin{equation}\label{eqObjdiff1}
    \frac{\partial D}{\partial \textbf{a}} = \sum_{j=1}^n 2(\frac{\partial \hat{\mathbf{p}}_{j}}{\partial \textbf{a}})^{T}(\hat{\mathbf{p}}_j - \mathbf{c}^{\mathcal{T}}_j)
\end{equation}

In this equation, the $\hat{\mathbf{p}}_{j}$ is the point on the calibrated surface and $\mathbf{c}_j$ is the closet point on the target model. The most important part is the $\frac{\partial \hat{\mathbf{p}}_{j}}{\partial \textbf{a}}^{T}$, which represents the calibrated point's gradient with respect to the actuation parameters. This information can be acquired by differentiating the neural deformation model as detailed in Appendix.\ref{Appendix:GradCompNerualDef}.

\subsection{Differentiation of Neural Deformation Model}\label{Appendix:GradCompNerualDef}

To calculate $\frac{\partial \hat{\mathbf{p}}_{j}}{\partial \textbf{a}}^{T}$, we have to take the analytical gradient of the RBF warping function Eq.\ref{equRBF}, two network differentiation (in Sec.\ref{secNeuralDefModel}) and B-Spline surface representation \cite{BSpline1974Book}. A pipeline has been drawn to clarify the relationship among variables:

\begin{figure}[h!] 
\centering
\includegraphics[width=0.9\linewidth]{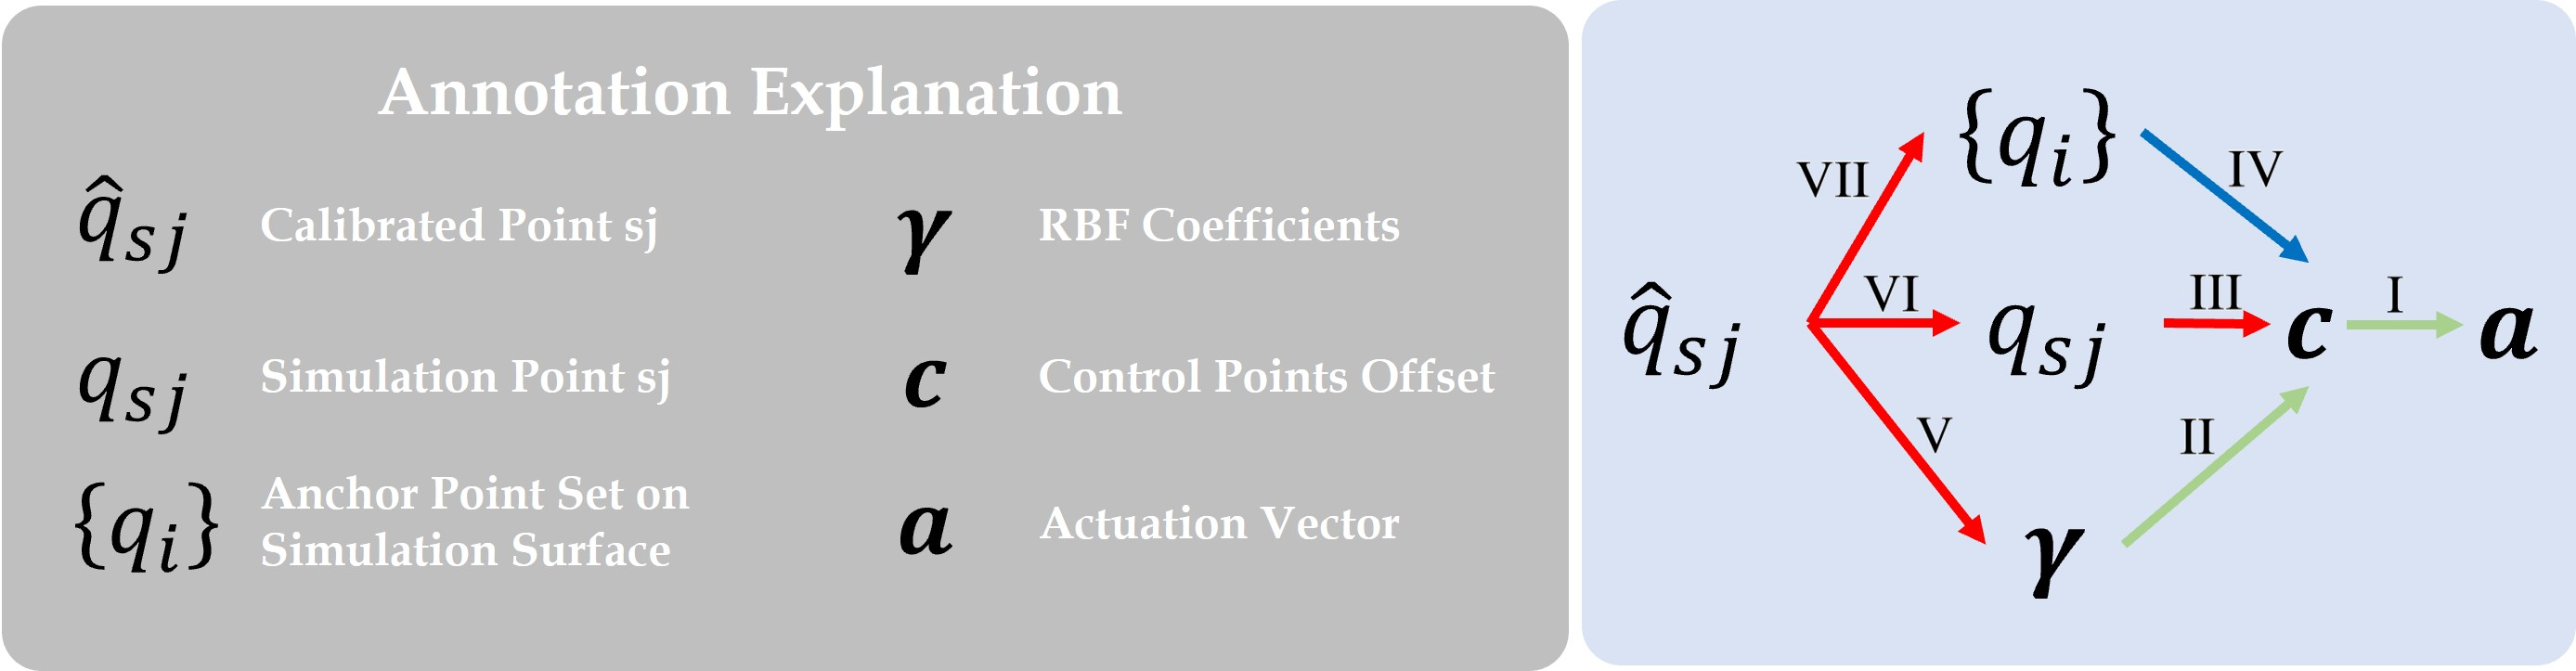}\\
\vspace{-2pt}
\caption{Left: the actual meaning of the variables used in the warping functions; Right: the chain rule applied to calculate the gradient of the variable $\hat{\mathbf{p}}_{sj}$ with respect to actutaion parameter $\textbf{a}$.
}\label{figVarRelation}
\end{figure}

In Fig.\ref{figVarRelation}, we use chain rule to calculate the gradient as follows:

\begin{flalign}
\label{eqCalPntGradient}
 % \begin{aligned}
\frac{\partial\mathbf{\hat{q}}_{sj}}{\partial \mathbf{a}} &= \frac{\partial\mathbf{\hat{q}}_{sj}}{\partial \{\mathbf{q}_i\}} \frac{\partial \{\mathbf{q}_i\}}{\partial \mathbf{c}} \frac{\partial \mathbf{c}}{\partial \mathbf{a}} + 
\frac{\partial \mathbf{\hat{q}}_{sj}}{\partial \mathbf{q}_{sj}} \frac{\partial \mathbf{q}_{sj}}{\partial \mathbf{c}} \frac{\partial \mathbf{c}}{\partial \mathbf{a}} + \frac{\partial\mathbf{\hat{q}}_{sj}}{\partial \bm{\gamma}} \frac{\partial \bm{\gamma} }{\partial \mathbf{c}} \frac{\partial \mathbf{c}}{\partial \mathbf{a}} \nonumber \\
&=(\frac{\partial\mathbf{\hat{q}}_{sj}}{\partial \{\mathbf{q}_i\}} \frac{\partial \{\mathbf{q}_i\}}{\partial \mathbf{c}}  + 
\frac{\partial \mathbf{\hat{q}}_{sj}}{\partial \mathbf{q}_{sj}} \frac{\partial \mathbf{q}_{sj}}{\partial \mathbf{c}} +
\frac{\partial\mathbf{\hat{q}}_{sj}}{\partial \bm{\gamma}} \frac{\partial \bm{\gamma} }{\partial \mathbf{c}}) \frac{\partial \mathbf{c}}{\partial \mathbf{a}} 
  %\end{aligned}
\end{flalign}

Note that $\{\mathbf{q}_i\}$ is a vector representing the collection of simulation marker coordinates with length as $3N$. $\bm{\gamma}$ stands for the combination of the RBF coefficients by sequentially flattening $\mathbf{a}_i$, $\mathbf{b}_i$ to be 1D vector with length as $3(N+4)$. For each gradient component in Eq.\ref{eqCalPntGradient}, we will describe the calculations one by one.

\subsubsection{Gradient of calibrated point to simulation marker points}

$\frac{\partial\mathbf{\hat{q}}_{sj}}{\partial \{\mathbf{q}_i\}}$ represents the gradient of the calibrated point $\mathbf{\hat{q}}_{sj}$ to simulation marker points $\{\mathbf{q}_i\}$ which can be back-propagated through Eq.\ref{equRBF}. The result is:

\begin{flalign}
\label{eqGradCalPnt2SimMarkers1}
\frac{\partial\mathbf{\hat{q}}_{sj}}{\partial \{\mathbf{q}_i\}} &=
\bigg[\begin{array}{c|c|c}
\frac{\partial\mathbf{\hat{q}}_{sj}}{\partial \mathbf{q}_1}
& \hdots{}
&\frac{\partial\mathbf{\hat{q}}_{sj}}{\partial \mathbf{q}_N}
\end{array}\bigg]
\\
\frac{\partial\mathbf{\hat{q}}_{sj}}{\partial \mathbf{q}_i} &=\mathbf{b}_i 
(\frac{\partial g(\mathopen| \mathbf{q}_{sj} - \mathbf{q}_{i} \mathclose|)}{\partial \mathbf{q}_i })^T
\end{flalign}

\begin{flalign}
\label{eqGradCalPnt2SimMarkers2}
\frac{\partial g(\mathopen| \mathbf{q}_{sj} - \mathbf{q}_{i} \mathclose|)}{\partial \mathbf{q}_i } = - \frac{\partial g(\mathopen| \mathbf{q}_{sj} - \mathbf{q}_{i} \mathclose|)}{\partial \mathopen| \mathbf{q}_{sj} - \mathbf{q}_{i} \mathclose|} \nonumber\\
\cdot((\mathbf{q}_{sj} - \mathbf{q}_{i})^T(\mathbf{q}_{sj} - \mathbf{q}_{i}))^{-\frac{1}{2}} (\mathbf{q}_{sj} - \mathbf{q}_{i}) 
\end{flalign}

\subsubsection{Gradient of calibrated point to the simulation query point}

$\frac{\partial \mathbf{\hat{q}}_{sj}}{\partial \mathbf{q}_{sj}}$ stands for the gradient of the calibrated point to the query point on the simulation surface and the result can be displayed as:

\begin{flalign}
\label{eqGradCalPnt2SimQueryPnt1}
\frac{\partial\mathbf{\hat{q}}_{sj}}{\partial \mathbf{q}_{sj}} &=
\mathbf{A} + 
\sum_{i=1}^{N} \mathbf{b}_i (\frac{\partial g(\mathopen| \mathbf{q}_{sj} - \mathbf{q}_{i} \mathclose|)}{\partial \mathbf{q}_{sj}})^T
\end{flalign}

\begin{flalign}
\label{eqGradCalPnt2SimQueryPnt2}
\frac{\partial g(\mathopen| \mathbf{q}_{sj} - \mathbf{q}_{i} \mathclose|)}{\partial \mathbf{q}_{sj}} = - \frac{\partial g(\mathopen| \mathbf{q}_{sj} - \mathbf{q}_{i} \mathclose|)}{\partial \mathbf{q}_i }
\end{flalign}

Note that Eq.\ref{eqGradCalPnt2SimQueryPnt2} only needs to change the sign of Eq.\ref{eqGradCalPnt2SimMarkers2}.

\subsubsection{Gradient of calibrated point to the RBF coefficients}

$\frac{\partial\mathbf{\hat{q}}_{sj}}{\partial \bm{\gamma}}$ is the gradient of the calibrated point to the query coefficients, which can be written as:

\begin{flalign}
\label{eqGradCalPnt2RBFCoeff1}
\frac{\partial\mathbf{\hat{q}}_{sj}}{\partial \bm{\gamma}} &=
\bigg[\begin{array}{c|c|c|c|c|c}
\frac{\partial\mathbf{\hat{q}}_{sj}}{\partial \mathbf{a}_0} &
\hdots&
\frac{\partial\mathbf{\hat{q}}_{sj}}{\partial \mathbf{a}_3} &
\frac{\partial\mathbf{\hat{q}}_{sj}}{\partial \mathbf{b}_1} &
\hdots
 &
\frac{\partial\mathbf{\hat{q}}_{sj}}{\partial \mathbf{b}_N} 
\end{array}\bigg]
\end{flalign}

\begin{align}
  \frac{\partial\mathbf{\hat{q}}_{sj}}{\partial \mathbf{a}_0} = \mathbf{I} &&
 \frac{\partial\mathbf{\hat{q}}_{sj}}{\partial \mathbf{a}_1} = (\mathbf{q}_{sj})_x\mathbf{I} &&
 \frac{\partial\mathbf{\hat{q}}_{sj}}{\partial \mathbf{a}_2} = (\mathbf{q}_{sj})_y\mathbf{I}  \nonumber
\end{align}

\begin{align}
\label{eqGradCalPnt2RBFCoeff2}
 \frac{\partial\mathbf{\hat{q}}_{sj}}{\partial \mathbf{a}_3} = (\mathbf{q}_{sj})_z\mathbf{I} &&
  \frac{\partial\mathbf{\hat{q}}_{sj}}{\partial \mathbf{b}_i} = g(\mathopen| \mathbf{q}_{sj} - \mathbf{q}_{i} \mathclose|) \mathbf{I}
\end{align}

In Eq.\ref{eqGradCalPnt2RBFCoeff2}, $(\mathbf{q}_{sj})_x$, $(\mathbf{q}_{sj})_y$ and $(\mathbf{q}_{sj})_z$ are the x, y and z component (scalar value) of the point $\mathbf{q}_{sj}$.

\subsubsection{Gradient of the simulation point to B-Spline control point offset}

$\frac{\partial \{\mathbf{q}_i\}}{\partial \mathbf{c}}$ and $\frac{\partial \mathbf{q}_{sj}}{\partial\mathbf{c}}$ are the gradient of the point on simulation surface with respect to control point offset $\mathbf{c}$ (flattened 1D vector).
According to B-Spline function:

\begin{flalign}
\label{eqBSplineFunc}
\mathbf{q}(u,v) = \sum_{i=1}^{N1}\sum_{j=1}^{N2} B_{ik}(u) B_{jl}(v) \mathbf{F}_{ij}
\end{flalign}
in this equation, $\mathbf{F}_{ij}$ is the control point with its gradient to control point offset is the identity matrix.
If we take gradient from $\mathbf{q}(u,v)$ to a specific control point offset vector (3D) $\mathbf{c}_{ij}$, we will get:
\begin{flalign}
\label{eqGradientBSpline}
\frac{\partial \mathbf{q}}{\partial \mathbf{c}_{ij}} = 
\frac{\partial \mathbf{q}}{\partial \mathbf{F}_{ij}}
\frac{\partial \mathbf{F}_{ij}}{\partial \mathbf{c}_{ij}} = 
B_{ik}(u) B_{jl}(v) \mathbf{I}
\end{flalign}

\subsubsection{Network Gradient}
$\frac{\partial \bm{\gamma} }{\partial \mathbf{c}}$ and $\frac{\partial \mathbf{c}}{\partial \mathbf{a}}$ can be easily acquired through the back-propagation of the RBF prediction network and Simulation FK Network.
