# Supplementary material for: Function based sim-to-real learning for shape control of deformable free-form surfaces
Source: arXiv:2405.08935 source file (2024-05-14)
Supplement: Supplementary file 2 [file secAppendix.tex]

\appendix
\subsection{Differentiation of Shape Approximation Loss}
 For Equ.\ref{eqPoseEstimation}, we want to calculate the gradient of the shape approximation loss $D(\mathcal{T}(\mathbf{R},\mathbf{t}),\mathcal{S}(\mathbf{a}))$
with respect to actuation parameter $\mathbf{a}$:

\begin{equation}\label{eqObjdiff1}
    \frac{\partial D}{\partial \textbf{a}} = \sum_{j=1}^n 2*(\frac{\partial \hat{\mathbf{p}}_{j}}{\partial \textbf{a}})^{T}(\hat{\mathbf{p}}_j - \mathbf{c}^{\mathcal{T}}_j)
\end{equation}

In this equation, the $\hat{\mathbf{p}}_{j}$ is the point on the calibrated surface and $\mathbf{c}_j$ is the closet point on the target model. The most important part is the $\frac{\partial \hat{\mathbf{p}}_{j}}{\partial \textbf{a}}^{T}$, which represents the calibrated point's gradient with respect to the actuation parameters. This information can be acquired by differentiating the neural deformation model as detailed in Appendix.\ref{Appendix:GradCompNerualDef}.

\subsection{Differentiation of Neural Deformation Model}\label{Appendix:GradCompNerualDef}

To calculate $\frac{\partial \hat{\mathbf{p}}_{j}}{\partial \textbf{a}}^{T}$, we have to take the analytical gradient of the RBF warping function Eq.\ref{equRBF}, two network differentiation (in Sec.\ref{secNeuralDefModel}) and B-Spline surface representation \cite{BsplinesurfacesConstruction}. A pipeline has been drawn to clarify the relationship among variables:

\begin{figure}[H] 
\centering
\includegraphics[width=0.9\linewidth]{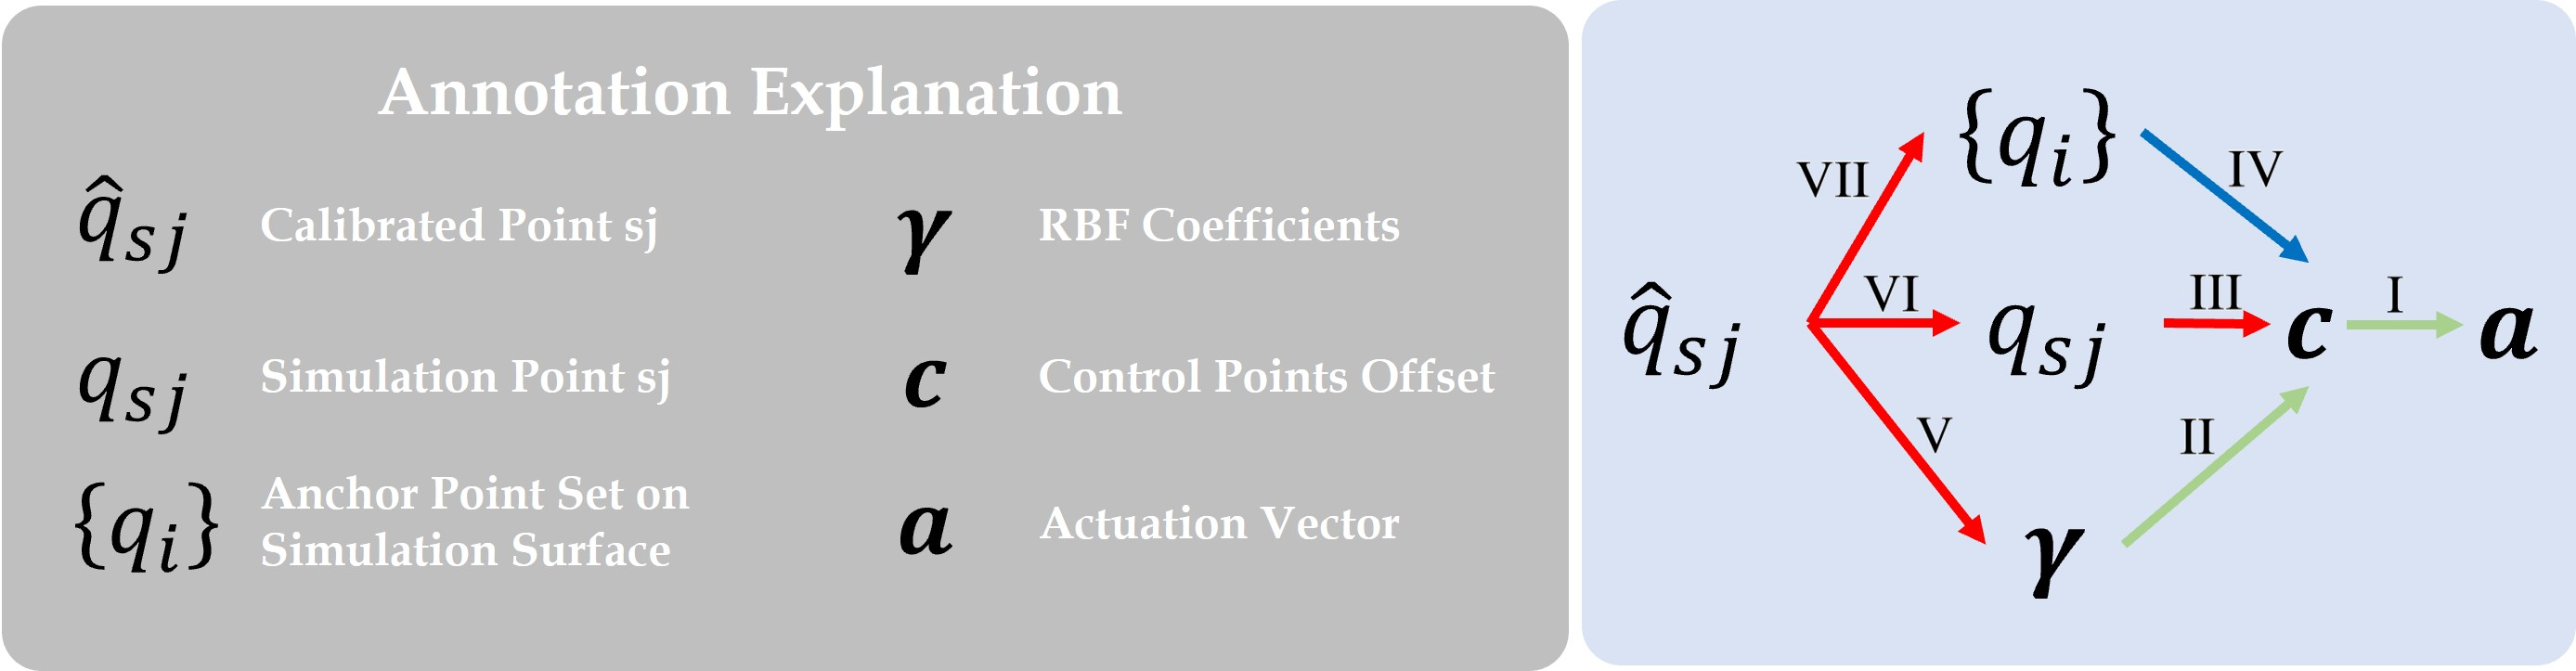}\\
\vspace{-2pt}
\caption{Left: the actual meaning of the variables used in the warping functions; Right: the chain rule applied to calculate the gradient of the variable $\hat{\mathbf{p}}_{sj}$ with respect to actutaion parameter $\textbf{a}$.
}\label{figVarRelation}
\end{figure}

In Fig.\ref{figVarRelation}, we use chain rule to calculate the gradient as follows:

\begin{equation}\label{eqDiffCalPnt2Act}
\frac{\partial\mathbf{\hat{q}}_{sj}}{\partial \mathbf{a}} = \frac{\partial\mathbf{\hat{q}}_{sj}}{\partial \{\mathbf{q}_i\}} \frac{\partial \{\mathbf{q}_i\}}{\partial \mathbf{c}} \frac{\partial \mathbf{c}}{\partial \mathbf{a}} + \frac{\partial \mathbf{\hat{q}}_{sj}}{\partial \mathbf{q}_{sj}} \frac{\partial \mathbf{q}_{sj}}{\partial \mathbf{c}} \frac{\partial \mathbf{c}}{\partial \mathbf{a}} + \frac{\partial\mathbf{\hat{q}}_{sj}}{\partial \bm{\gamma}} \frac{\partial \bm{\gamma} }{\partial \mathbf{c}} \frac{\partial \mathbf{c}}{\partial \mathbf{a}}
\end{equation}
